# Supplementary material for: Stacking-Dependent Van Hove Singularity Shifts in Three-Dimensional Charge Density Waves of Kagome Metals AV$_3$Sb$_5$ (A = K, Rb, Cs)
Source: arXiv:2408.10402 source file (2024-08-28)
Supplement: Supplementary file 1 [file SI.pdf]

# Supplemental Information for
# *"Stacking-Dependent Van Hove Singularity Shifts in Three-Dimensional Charge Density Waves of Kagome Metals $AV_3Sb_5$ ($A$ = K, Rb, Cs)"*

Chanchal K. Barman[1,*], Sun-Woo Kim[2,*], Youngkuk Kim[1,†]

[1] *Department of Physics, Sungkyunkwan University, Suwon 16419, Korea*

[2] *Department of Materials Science and Metallurgy, University of Cambridge, 27 Charles Babbage Road, Cambridge, United Kingdom*

## Contents

**Tight-binding Hamiltonian** 2

**Dispersion near the type-II van Hove singularities from TB Hamiltonian** 6

## TIGHT-BINDING HAMILTONIAN

In this section, we provide a detailed description of each matrix term in our tight-binding (TB) Hamiltonian. Schematic representations of the nearest neighbor (NN), next-nearest neighbor (NNN) hopping within the 2D kagome layer, and interlayer hopping between the vertically stacked kagome layers are illustrated in Fig. S1. Considering a basis set $\Psi_k^T = \left(A_k^T, B_k^T, C_k^T\right)$ and $\alpha_k^T = (\alpha_{1,k}, \alpha_{2,k}, \alpha_{3,k}, \alpha_{4,k})$, where $\alpha_i$ represents sublattice index for vanadium sites in the $2 \times 2$ unit cell as shown in Fig. S1, we express the hopping matrices as follows:

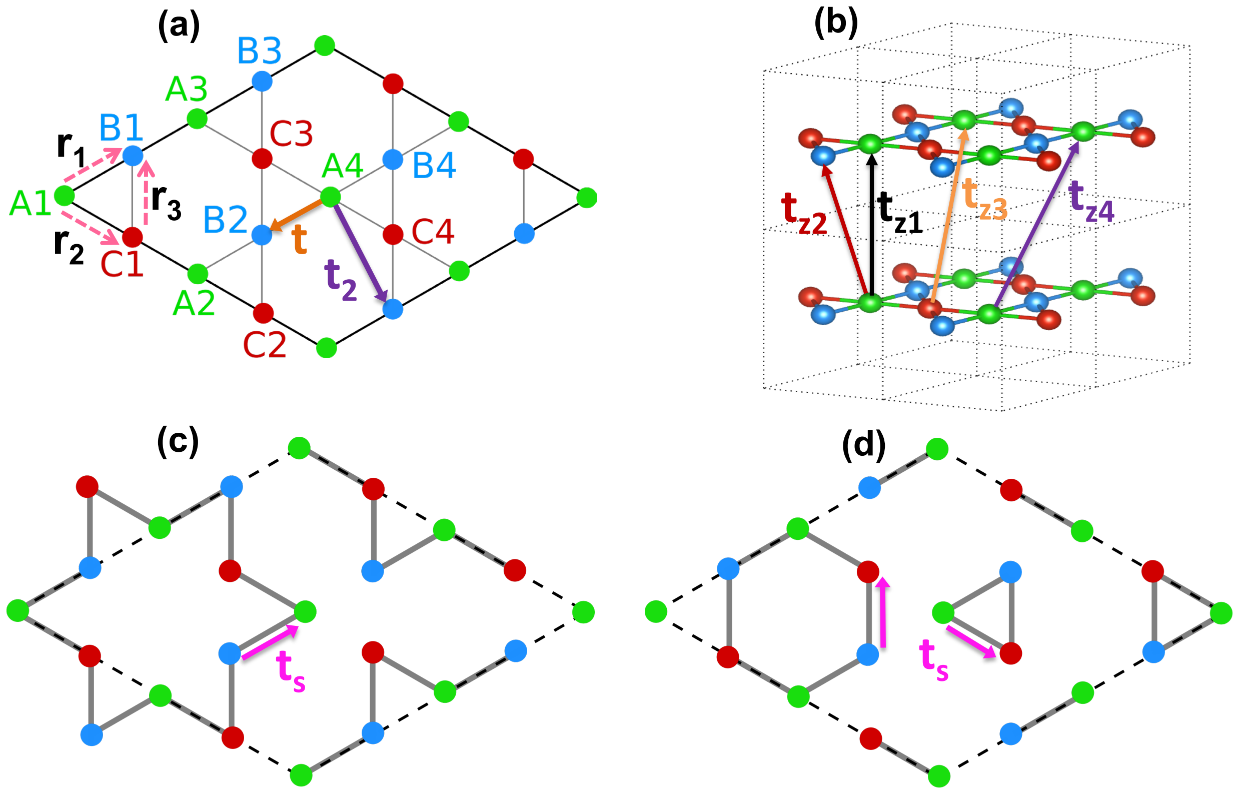


FIG. S1: (Color online) (a) $2 \times 2$ unit cell with sublattice indices. $t$ and $t_2$ are NN and NNN hopping strength. (b) Kagome layers stacked along $z$-direction. $t_{z1}$, $t_{z2}$, $t_{z3}$, and $t_{z4}$ are NN, NNN, NNNN, and NNNNN hopping strengths along $z$-direction. (c,d) CDW structure with SD and ISD distortion.

$$
\mathcal{H}_{NN}(\mathbf{k}) = -t \begin{pmatrix}
\varepsilon & 0 & 0 & 0 & \phi_1 & 0 & \phi_1^* & 0 & \phi_2 & \phi_2^* & 0 & 0 \\
 & \varepsilon & 0 & 0 & 0 & \phi_1 & 0 & \phi_1^* & \phi_2^* & \phi_2 & 0 & 0 \\
 & & \varepsilon & 0 & \phi_1^* & 0 & \phi_1 & 0 & 0 & 0 & \phi_2 & \phi_2^* \\
 & & & \varepsilon & 0 & \phi_1^* & 0 & \phi_1 & 0 & 0 & \phi_2^* & \phi_2 \\
 & & & & \varepsilon & 0 & 0 & 0 & \phi_3^* & 0 & 0 & \phi_3 \\
 & & & & & \varepsilon & 0 & 0 & 0 & \phi_3^* & \phi_3 & 0 \\
 & & & & & & \varepsilon & 0 & 0 & \phi_3 & \phi_3^* & 0 \\
 & & h.c. & & & & & \varepsilon & \phi_3 & 0 & 0 & \phi_3^* \\
 & & & & & & & & \varepsilon & 0 & 0 & 0 \\
 & & & & & & & & & \varepsilon & 0 & 0 \\
 & & & & & & & & & & \varepsilon & 0 \\
 & & & & & & & & & & & \varepsilon
\end{pmatrix} \tag{S1}
$$

$$
\mathcal{H}_{NNN}(\mathbf{k}) = -t_2 \begin{pmatrix}
0 & 0 & 0 & 0 & 0 & \phi_6^* & 0 & \phi_6 & 0 & 0 & \phi_5^* & \phi_5 \\
 & 0 & 0 & 0 & \phi_6^* & 0 & \phi_6 & 0 & 0 & 0 & \phi_5 & \phi_5^* \\
 & & 0 & 0 & 0 & \phi_6 & 0 & \phi_6^* & \phi_5^* & \phi_5 & 0 & 0 \\
 & & & 0 & \phi_6 & 0 & \phi_6^* & 0 & \phi_5 & \phi_5^* & 0 & 0 \\
 & & & & 0 & 0 & 0 & 0 & 0 & \phi_4^* & \phi_4 & 0 \\
 & & & & & 0 & 0 & 0 & \phi_4^* & 0 & 0 & \phi_4 \\
 & & & & & & 0 & 0 & \phi_4 & 0 & 0 & \phi_4^* \\
 & & h.c. & & & & & 0 & 0 & \phi_4 & \phi_4^* & 0 \\
 & & & & & & & & 0 & 0 & 0 & 0 \\
 & & & & & & & & & 0 & 0 & 0 \\
 & & & & & & & & & & 0 & 0 \\
 & & & & & & & & & & & 0
\end{pmatrix} \tag{S2}
$$

$$
\mathcal{H}_{ISD}(\mathbf{k}) = -t_s
\begin{pmatrix}
0 & 0 & 0 & 0 & 0 & 0 & \phi_1^* & 0 & 0 & \phi_2^* & 0 & 0 \\
 & 0 & 0 & 0 & 0 & \phi_1 & 0 & 0 & \phi_2^* & 0 & 0 & 0 \\
 & & 0 & 0 & \phi_1^* & 0 & 0 & 0 & 0 & 0 & \phi_2 & 0 \\
 & & & 0 & 0 & 0 & 0 & \phi_1 & 0 & 0 & 0 & \phi_2 \\
 & & & & 0 & 0 & 0 & 0 & \phi_3^* & 0 & 0 & 0 \\
 & & & & & 0 & 0 & 0 & 0 & 0 & \phi_3 & 0 \\
 & & & & & & 0 & 0 & 0 & \phi_3 & 0 & 0 \\
 & & h.c. & & & & & 0 & 0 & 0 & 0 & \phi_3^* \\
 & & & & & & & & 0 & 0 & 0 & 0 \\
 & & & & & & & & & 0 & 0 & 0 \\
 & & & & & & & & & & 0 & 0 \\
 & & & & & & & & & & & 0
\end{pmatrix}
\tag{S3}
$$

$$
\mathcal{H}_{SD}(\mathbf{k}) = -t_s
\begin{pmatrix}
0 & 0 & 0 & 0 & \phi_1 & 0 & 0 & 0 & \phi_2 & 0 & 0 & 0 \\
 & 0 & 0 & 0 & 0 & 0 & 0 & \phi_1^* & 0 & \phi_2 & 0 & 0 \\
 & & 0 & 0 & 0 & 0 & \phi_1 & 0 & 0 & 0 & 0 & \phi_2^* \\
 & & & 0 & 0 & \phi_1^* & 0 & 0 & 0 & 0 & \phi_2^* & 0 \\
 & & & & 0 & 0 & 0 & 0 & 0 & 0 & 0 & \phi_3 \\
 & & & & & 0 & 0 & 0 & 0 & \phi_3^* & 0 & 0 \\
 & & & & & & 0 & 0 & 0 & 0 & \phi_3^* & 0 \\
 & & h.c. & & & & & 0 & \phi_3 & 0 & 0 & 0 \\
 & & & & & & & & 0 & 0 & 0 & 0 \\
 & & & & & & & & & 0 & 0 & 0 \\
 & & & & & & & & & & 0 & 0 \\
 & & & & & & & & & & & 0
\end{pmatrix}
\tag{S4}
$$

$$\mathcal{H}^{3D}_{NN}(\mathbf{k}) \;=\; -2t_{z1}\,\phi_z\,\mathbb{I}_{12} \tag{S5}$$

$$\mathcal{H}^{3D}_{NNN}(\mathbf{k}) \;=\; -t_{z2}\,\phi_z\,\mathcal{H}_{NN}(\mathbf{k}) \tag{S6}$$

$$\mathcal{H}^{3D}_{NNNN}(\mathbf{k}) \;=\; -t_{z3}\,\phi_z\,\mathcal{H}_{NNN}(\mathbf{k}) \tag{S7}$$

$$\mathcal{H}^{3D}_{NNNNN}(\mathbf{k}) \;=\; -t_{z4}\,\mathbb{I}_3 \otimes \Lambda \tag{S8}$$

$$\Lambda = 2\phi_z \begin{pmatrix} 0 & \cos(\mathbf{k}\cdot\nu_{\mathbf{9}}) & \cos(\mathbf{k}\cdot\nu_{\mathbf{8}}) & \cos(\mathbf{k}\cdot\nu_{\mathbf{7}}) \\ & 0 & \cos(\mathbf{k}\cdot\nu_{\mathbf{7}}) & \cos(\mathbf{k}\cdot\nu_{\mathbf{8}}) \\ & h.c. & 0 & \cos(\mathbf{k}\cdot\nu_{\mathbf{9}}) \\ & & & 0 \end{pmatrix} \tag{S9}$$

In the above, $\mathbb{I}_3$ and $\mathbb{I}_{12}$ are $3 \times 3$ and $12 \times 12$ identity matrices respectively and $\varepsilon$ is the onsite energy. The notations, $\phi_j = e^{i\mathbf{k}\cdot\mathbf{r_j}}$ for $j \in (1,3)$ and $\phi_j = e^{i\mathbf{k}\cdot\nu_{\mathbf{j}}}$ for $\nu \in (4,6)$, $\phi_z = \cos(\mathbf{k}\cdot\mathbf{r_z})$ and the position vectors are $\mathbf{r_1} = \frac{1}{2}(\sqrt{3},1)$, $\mathbf{r_2} = \frac{1}{2}(\sqrt{3},-1)$, $\mathbf{r_3} = (0,1)$ $\nu_{\mathbf{4}} = \mathbf{r_1} + \mathbf{r_2}$, $\nu_{\mathbf{5}} = \mathbf{r_1} + \mathbf{r_3}$, $\nu_{\mathbf{6}} = \mathbf{r_2} - \mathbf{r_3}$, $\nu_{\mathbf{7}} = 2\mathbf{r_3}$, $\nu_{\mathbf{8}} = 2\mathbf{r_1}$, $\nu_{\mathbf{9}} = 2\mathbf{r_3}$, $\mathbf{r_z} = (0,0,c_z)$. Here, $c_z = 1.643$, $1.680$, $1.715$ for $KV_3Sb_5$, $RbV_3Sb_5$, and $CsV_3Sb_5$ respectively.

## DISPERSION NEAR THE TYPE-II VAN HOVE SINGULARITIES FROM TB HAMILTONIAN

In this section, using the TB Hamiltonian we present an effective low-energy expansion of the dispersion around the vicinity of the type-II VHSs, as illustrated in Fig. 2 of the main manuscript. The expression for the dispersion polynomial is detailed in Eq. (S10). $k_x$ and $k_y$ are crystal momenta relative to the VHS point. Details about the various parameters in the dispersion are listed in Table S1.

$$E_k = \varepsilon_0 + \alpha k_y + \beta_1 k_x^2 + \beta_2 k_y^2 + \gamma_1 k_y^3 + \gamma_2 k_x^2 k_y + \delta_1 k_x^4 + \delta_2 k_y^4 + \delta_3 k_x^2 k_y^2 \tag{S10}$$

TABLE S1: Various parameters of the dispersion in Eq. (S10). The unit of $\varepsilon_0$, $\alpha$, $\beta_i$, $\gamma_i$ and $\delta_i$ are given in eV, eV.Å, eV.Å$^2$, eV.Å$^3$, and eV.Å$^4$ respectively.

| | $\varepsilon_0$ | $\alpha$ | $\beta_1$ | $\beta_2$ | $\gamma_1$ | $\gamma_2$ | $\delta_1$ | $\delta_2$ | $\delta_3$ |
|---|---|---|---|---|---|---|---|---|---|
| $CsV_3Sb_5$ | -0.0346 | 0.0001 | 0.1949 | -0.4190 | 0.9303 | -0.7292 | -2.3940 | 0.5209 | 5.3077 |
| $KV_3Sb_5$ | -0.0069 | -0.0068 | 0.6582 | -0.6517 | 0.3313 | -2.0620 | -5.5080 | 2.1522 | 2.7612 |
| $RbV_3Sb_5$ | -0.0288 | 0.0107 | 0.5389 | -0.6531 | 0.4393 | -1.8213 | -4.3305 | 1.9734 | 4.3466 |
